# Supplementary material for: EpiDiff: Enhancing Multi-View Synthesis via Localized Epipolar-Constrained Diffusion
Source: arXiv:2312.06725 source file (2024-04-02)
Supplement: Supplementary file 1 [file X_suppl.tex]

\clearpage
\setcounter{page}{1}
\maketitlesupplementary

\section{Rationale}

Epipolar Geometry, a fundamental concept in computer vision and photogrammetry, describes the geometric relationship between the viewpoints of two cameras and a point in a scene. This geometry is pivotal in understanding how the position of a point in one camera view constrains its position in the other view.

In epipolar geometry, each camera's center and a scene point form a line. This line projects onto the imaging plane of the other camera as an "epipolar line". A critical aspect of epipolar geometry is that if the position of a scene point is known in one camera view, its position in the other view must lie along the corresponding epipolar line.

Formally, let \(\mathbf{P}\) be a point in 3D space, and \(\mathbf{C}_1\) and \(\mathbf{C}_2\) be the centers of two cameras. The projection of \(\mathbf{P}\) onto the image planes of the cameras are \(\mathbf{p}_1\) and \(\mathbf{p}_2\) respectively. The epipolar constraint can be mathematically represented as:

\begin{align}
    \mathbf{p}_2^T \mathbf{F} \mathbf{p}_1 = 0
\end{align}

where \(\mathbf{F}\) is the fundamental matrix, a 3x3 matrix that encapsulates the intrinsic and extrinsic parameters of the cameras. The rows of \(\mathbf{F}\) correspond to the coefficients of the epipolar lines in the second camera's image plane.

Additionally, epipolar geometry involves the concepts of epipoles and epipolar planes. Epipoles are the points of intersection of all epipolar lines in the image plane, and the epipolar plane is defined by the line connecting \(\mathbf{C}_1\) and \(\mathbf{C}_2\) and the point \(\mathbf{P}\). These geometric constructs provide a theoretical foundation for understanding and implementing complex visual tasks such as stereo vision and 3D reconstruction.
